# Supplementary material for: From Trees to Continuous Embeddings and Back: Hyperbolic Hierarchical Clustering
Source: arXiv:2010.00402 source file (2020-10-01)
Supplement: Supplementary file 1 [file decoding.tex]

We now focus our attention on the difference between the continuous and discrete cost during decoding. 
We show that if the optimization returns an embedding $Z$ that is close to a tree metric, then its cost is close to the optimal Dasgupta cost.
That is, if it is $\varepsilon$-distortion with respect to some tree $T$, then the previous the continuous cost of $Z$ equals the discrete cost of $T$, up to some continuous error approximation. 

\cref{lemma:lca_agreement} states that if $Z$ is $\varepsilon$-relative metric for a tree $T$ and $\varepsilon$ is sufficiently small, then $Z$ and $T$ are in LCA agreement.
We use this result to show that if the embeddings represent a $\varepsilon$-relative metric of a binary tree metric, then the decoding~\cref{alg:decoding} will recover the underlying discrete tree perfectly~(\cref{lemma:decoding}). 
We then prove a bound on the difference between the continuous cost and the discrete cost of a decoded tree~(\cref{lemma:decoding}). 

%\decoding*
\input{figures/tikz_decoding_proof}
\begin{proof}
We consider the case where $T$ is binary and discuss the non-binary case in~\cref{remark:non_binay}.
We show the result by strong induction on the different steps ($s$) of the decoding algorithm.
For $\varepsilon$ sufficiently small, $T$ and $Z$ are in LCA agreement as per~\cref{lemma:lca_agreement}.
Therefore, the ordering of pairwise LCA distances in $T$ and $Z$ is the same. 
Therefore, it suffices to show that having access to the exact ordering of all pairwise leaves' LCA distances to the root $r$ in $T$, one can recover the exact tree using~\cref{alg:decoding}.

{$\mathbf{s=1}$}: The largest LCA distance to the root is achieved for a pair of sibling leaves (otherwise we could show by contradiction that there exist another pair with a larger distance to the root).  
Therefore, for $s=1$, the decoding algorithm merges a correct pair of sibling leaves in $T$. 

{$\mathbf{s\ge2}$}: 
Now suppose $s\ge2$ and assume that so far all subtrees in the forest $F$ in~\cref{alg:decoding} exactly match the corresponding subtree in $T$. 
Let $(i, j)$ be the next pair chosen by the algorithm, let $(T_i, T_j)$ denote the corresponding subtrees in $F$ (these could also be isolated nodes if this is the first time that $i$ or $j$ is picked by the algorithm), and let $(r_i, r_j)$ denote the roots of $(T_i, T_j)$ respectively~(\cref{fig:decoding_proof}). 
Since $(i, j)$ was picked by the algorithm, we get that:
\begin{align}\label{eq:decoding_proof}
        d_T(r, i\vee j)&\ge d_T(r, i\vee k) & \forall k\in\mathrm{leaves}(T)\setminus\mathrm{leaves}(T_i),\\
    d_T(r, i\vee j)&\ge d_T(r, j\vee k)& \forall k\in\mathrm{leaves}(T)\setminus\mathrm{leaves}(T_j).
\end{align}
We claim that this implies that $(r_i, r_j)$ must be siblings in $T$ and show this by contradiction. 
Assume that there exist another node $r_k\notin T_i\cup T_j$ (not necessarily a leaf node) such that $(r_i, r_k)$ are sibling in $T$ and let $k$ be a leaf descendant of $r_k$ (or $r_k$ itself if $r_k$ is a leaf in $T$). 
Since $(r_i, r_k)$ are siblings, and since $r_j$ is not a descendant of $r_i$ nor a descendant of $r_k$, we have:
\begin{align*}
    d_T(r, i\vee k) = d_T(r, r_i\vee r_k) > d_T(r, r_i\vee r_j) = d_T(r, i\vee j). 
\end{align*}
Therefore $d_T(r, i\vee k)>d_T(r, i\vee j)$ which contradicts~(\cref{eq:decoding_proof}).
Therefore the algorithm picked the right pair at step $s$ which end the induction proof. 
\end{proof}
\begin{remark}\label{remark:non_binay}
Note that the previous result applies only if $Z$ is the low-distortion embedding of a binary tree. 
If $Z$ is the low-distortion embedding of a non-binary tree, then~\cref{alg:decoding} outputs a ``caterpilar-like'' binary tree where each intermediate node with more than two children is split into multiple nodes of degree two~(\cref{fig:binary_decoding}). 
The non-binary tree is at least as costly as the binary tree as per Section 2.3 in~\cite{dasgupta2016cost}, and we use this fact to show our main result for general tree metric embddings. 
\end{remark}
